# Supplementary material for: Towards Heisenberg limit without critical slowing down via quantum reinforcement learning
Source: arXiv:2503.02210 source file (2025-03-04)
Supplement: Supplementary file 1 [file criticalsensing_prl_sm.pdf]

# SUPPLEMENTARY MATERIAL
# Towards Heisenberg limit without critical slowing down via quantum reinforcement learning

Hang Xu,[1] Tailong Xiao,[1,2,3] Jingzheng Huang,[1,2,3] Ming He,[4] Jianping Fan,[4] and Guihua Zeng[1,2,3]

[1]*State Key Laboratory of Advanced Optical Communication Systems and Networks, Institute for Quantum Sensing and Information Processing, Shanghai Jiao Tong University, Shanghai 200240, P.R. China*
[2]*Hefei National Laboratory, Hefei, 230088, P.R. China*
[3]*Shanghai Research Center for Quantum Sciences, Shanghai, 201315, P.R. China*
[4]*AI Lab, Lenovo Research, Beijing 100094, P.R. China*

## I. QUANTUM DQN ALGORITHM

In this section, we detail the DQN algorithm and optimization process for our QRL. Q-learning is a classical RL algorithm for solving the optimal action selection problem in Markov decision making process. The core idea is to determine which action to take in a given state maximizes the long-term cumulative reward by estimating the value function $Q(s,a)$ (expectation of the gain that can be obtained by taking action $a$ in state $s$ at a given moment in time) for each state-action pair. While Q-learning is theoretically effective, its implementation in tabular form becomes impractical when dealing with high-dimensional state spaces or continuous action spaces. To address this problem, some work has begun to explore the use of function approximation methods to approximate Q functions. This led to the concept of DQN. DQN combine Q-learning with deep neural networks, enabling them to handle complex environments and state spaces while maintaining an efficient estimate of the value function.

DQN is a deep RL algorithm designed to solve value-based RL problems. The basic idea is to utilize deep neural networks to approximate value functions for learning optimal action strategies for the environment.The DQN algorithm combines the strengths of deep learning and RL and has achieved significant success in complex environments such as video games. Based on Q-learning, DQN proposes two techniques to make the Q-network update iteration more stable. (i) Experience Replay: Use a pool of experience to store multiple experiences $(s_t, a_t, r_t, s_{t+1})$, and then randomly select a batch of data from it for training. (ii) Fixed Q-Target: Replicate a target that has the same structure as the original Q-network. Target-Q network with the same structure as the original Q-network, which is used to compute the Q-target value.

The original DQN algorithm uses temporal difference (TD) learning to update the parameters of the Q function. The network parameters are updated by minimising the difference between the current estimated Q value and the target Q value calculated based on the TD target. The procedure is as follows: (1) Initialize the network, input the state $s_t$, and output the Q values of all actions under $s_t$; (2) Using a strategy (e.g. $\varepsilon$-greedy), select an action $a_t$, input $a_t$ to the environment, and obtain the new states $s_{t+1}$ and $r_t$; (3) Calculate the TD target: $y_t = r_t + \gamma \cdot \mathrm{argmax}_a Q(s_{t+1}, a; w)$; (4) Calculate the loss function: $L = [y_t - Q(s,a;w)]^2$; (5) Update the Q parameters so that $Q(s_t, a_t)$ is as close as possible to $y_t$, using gradient descent to do the updating; 6. feed $s_t$ into the network and repeat the previous process.

The original DQN algorithm is prone to overestimation problems, which can be mitigated to some extent by using the target network [1]. Here the two networks have different roles: the evaluation network $Q(s,a;w)$ is responsible for controlling the intelligentsia and collecting experience; the target network $Q(s,a;\bar{w})$ is used to compute the TD target:

$$y_t = r_t + \gamma \cdot \mathrm{argmax}_a Q(s_{t+1}, a; \bar{w}). \tag{S1}$$

During the update process, only the weights of the evaluation network $Q(s,a;w)$ are updated, and the weights of the target network $Q(s_{t+1},a;\bar{w})$ remain unchanged. After a certain number of updates, the weights of the updated evaluation network are then copied to the target network for the next batch of updates. The introduction of the target network increases the stability of the learning since the target values of the returns are relatively fixed over a period of time when the target network does not change.

The introduction of the target network mitigates the overestimation problem to some extent, but there is still a maximisation operation and the overestimation problem is still significant. To further address the overestimation problem, the double DQN algorithm was proposed [2]. Compared to the previously introduced DQN using target network in Eq. (S1), the improvement of the double DQN lies in the computation of the TD target, which uses the original network $Q(s,a;w)$ to select the one that maximises the Q value, denoted as $a^*$, and then uses the target network to compute the target value by using this $a^*$, i.e., $y_t = r_t + \gamma \cdot Q(s_{t+1}, a^*; \bar{w})$. Notice that

$$Q(s_{t+1}, a^*; \bar{w}) < \mathrm{argmax}_a Q(s_{t+1}, a; \bar{w}), \tag{S2}$$

which leads to the overestimation being further mitigated. In this work, we use the double DQN algorithm and in addition the network has quantum features (it contains quantum circuits). The detailed procedure of the algorithm we use is shown in Algorithm 1. Here for $L = 30$, the hyper-parameters we set are $T = 50, N_{eps} = 40000, n_{batch} = 32, \gamma = 0.98, N_{pool} = 8000, n_{tar} = 10$, and $\varepsilon_1 = 1$.

**Algorithm 1** Quantum reinforcement learning

**Require:** Target state $\psi^*$, target fidelity $F^*$, maximum episode length $T$, number of training episodes $N_{eps}$, learning rate $\eta$, batch size $n_{batch}$, discount factor $\gamma$, experience pool size $N_{pool}$, target network update frequency $n_{tar}$, and initial exploration parameter $\varepsilon_1$.

```
Randomly initialise the Q-network with weights w,and copy it to the target Q-network with w̄ ← w
Phase 1: Collecting experience
for i = 1 → N_pool do
    Reset the RL environment and sample the initial state ψ
    Choose a random action a and impose it on the environment (spin chain) to make it undergo unit evolution to a new
    state ψ′
    Compute the reward function r and add the transition (ψ, a, r, ψ′) to the experience pool
end for
Phase 2: Training
for j = 1 → N_eps do
    Reset the RL environment and return to the initial state ψ_0
    Get recession exploration parameter: ε_j = ε_1 e^{−j/N_eps}
    for t = 1 → T do
        Phase 2.1: Update network parameters
        Sample n_batch transitions (ψ, a, r, ψ′) from the experience pool
        Based on initial and target networks calculate TD target: y = r + γ · Q(ψ′, a*; w̄)
        Compute the gradient of the loss function L = Σ_batch (y − Q(ψ, a; w))^2 with respect to the network parameter θ
        Update original Q network with gradient descent based on learning rate η
        Copy the parameters to the target-Q network every n_tar updates of the original Q network w̄ ← w
        Phase 2.2: Update environment (evolution of spin chain)
        Select control action a_t based on ε_t-greedy strategy
        Environment (spin chain) undergoes time evolution to a new state ψ_{t+1}
        Compute the reward function r_t and add the transition (ψ_t, a_t, r_t, ψ_{t+1}) to the experience pool
        if r_t < log F*,then break
    end for
end for
```

## II. PREPARATION CRITICAL PROBES VIA QRL

The preparation of quantum states using RL is typically modeled as a Markov decision process, where the agent interacts with the environment. The environment is described by the quantum system and its dynamics. In each training episode, the agent first obtains observable measurements of the quantum system from the environment. Based on these measurements, the agent applies control actions to the quantum state in the environment, causing it to evolve to a new state, and so on, until the maximum number of steps $T$ is reached. During this process, the agent collects reward signals for each step, with the goal of finding the optimal control strategy that maximizes the total return for the entire episode.

Here, we set that only a number of fixed gate operations can be applied to the quantum state in the maximum time to maximize the target state fidelity, which is actually a combinatorial optimization problem. Choosing an appropriate reward function helps the network to converge quickly during the training process, and for a state preparation task, the most intuitive choice is the target state fidelity, and of course the entanglement entropy and the energy can also be made as the reward function for a specific task.

Noting that driving a many-body spin chain requires more one- and two-site gate operations, here we use apply the value-based deep Q-network (DQN) algorithm, which handles large state spaces well and yields long-term payoffs, saves data and speeds up the agent convergence to the optimum more than the policy-based algorithm. Therefore, here we select the global single- and two-site Pauli gate lasting for a fixed time $\pm\delta t$ as the action space of the environment, i.e.,

$$\mathcal{A} = \{X, Y, Z, XX, YY, ZZ\}, \tag{S3}$$

where $X, Y, Z = e^{\pm i\delta t \sum \sigma_i^{x,y,z}}$ and $XX, YY, ZZ = e^{\pm i\delta t \sum \sigma_i^{x,y,z}\sigma_{i+1}^{x,y,z}}$. Since the entanglement of the many-body ground

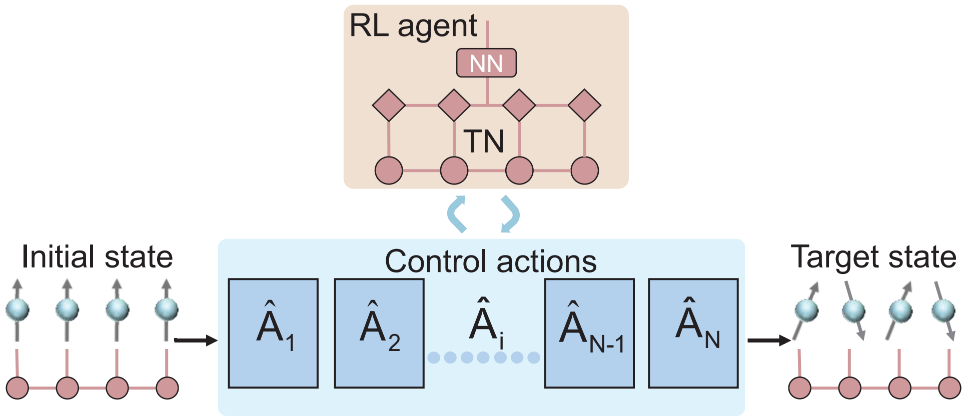


FIG. S1. Schematic of the agent-environment interaction process in QRL. The agent consists of a tensor network or quantum circuit and a classical fully connected network, and the environment consists of a spin chain and its evolutionary approach. At each step in the training process, the agent evaluates the current state of the spin chain and outputs a control action to the spin chain, where the control action is a discrete-time unitary quantum gate. The agent's task is to control the evolution of the spin chain from the initial state to the target critical ground state.

state satisfies the area law [3], the use of matrix product state (MPS) [4, 5] characterization can greatly compress its information, so here we use the MPS as the characterization of quantum states in the environment and input for agent. Naturally, in order to receive the characterization of the MPS, the agent consists of a parameter-containing quantum circuit and a fully-connected network, which is the quantum feature that distinguishes our algorithm from the classical DQN algorithm. In addition, to motivate the agent to use as few gate operations as possible to reach the target fidelity, we choose $r_t = \log F_t$ as the reward function, where $F_t$ is the fidelity of the quantum state in an episode to the target state after the $t_i$ step. The return obtained as an entire episode is $R = \sum_{t=1}^{T} r_t$, where $T = 50$ is the maximum allowed episode length. Noting that the return is always negative, it is clear that the smaller the number of moves required to maximize the return while achieving the target fidelity. In Fig. S1, we show a schematic of the agent-environment interaction using quantum RL to manipulate the many-body system.

In order to further reduce the exploration space of the agent, we first train the agent to prepare spin-chain ($L = 8$) ground states, and find that all the gate operations required in the optimal preparation scheme that eventually converges are a subset of Eq. (S3), i.e., $\{X, Z, YY, ZZ\}$. Finally, we use this set of gate operations as the agent's action space for the preparation of intermediate-scale ($L = 30$) spin-chain ground states with total fidelity threshold $F^*$ (corresponding single-particle fidelity threshold $F_{sp}^* = \sqrt[30]{F^*} = 0.995$).

## III. MATRIX PRODUCT STATES (MPS)

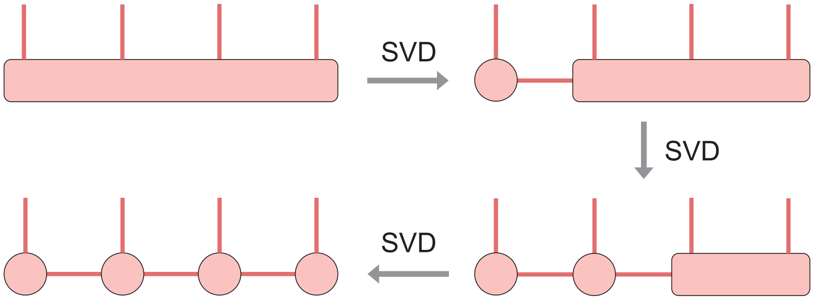


FIG. S2. Schematic of SVD decomposition of a tensor. For a wave function describing a quantum state of $L$ lattice points, the probability amplitude is an $L$-order tensor. In each SVD, the fraction of low singular values is truncated, and the final $L$-order tensor is decomposed into a product of $L$ matrices, i.e., the MPS.

Considering a one-dimensional system consisting of $L$ lattice points, each of which is occupied by a 1/2-spin with Hilbert space dimension $d = 2$, the arbitrary wave function of this lattice system can be expressed as

$$|\psi\rangle = \sum_{i_1 i_2 \cdots i_L} \psi_{i_1 i_2 \cdots i_L} |i_1 i_2 \cdots i_L\rangle, \tag{S4}$$

where $\psi$ is a tensor with $L$ indicators or dimensions as well as $i_j = \{0_j, 1_j\}$ is the state of the $j$-th spin (also called the physical dimension). It is easy to show that $\psi$ can be decomposed into a product of $L$ matrices, i.e.:

$$\psi_{i_1 i_2 \cdots i_L} = \sum_{s_1 s_2 \cdots s_L} A^{(1)}_{i_1 s_1} A^{(2)}_{s_1 i_2 s_2} A^{(3)}_{s_2 i_3 s_3} \cdots A^{(L)}_{s_{L-1} i_L s_L}, \tag{S5}$$

this process is accomplished by performing a singular value decomposition (SVD) of $\psi$ (as shown in Fig. S2). For $A^{(j)}_{s_{j-1} i_j s_j}$, $i_j$ is the physical dimension of the $j$-th spin and $s_l$ is the virtual dimension (bond dimension), it can be viewed as entanglement with neighboring spins.

Notice that the representations on the left and right sides in Eq. S5 are essentially the same, and their complexity in describing the chain of spins grows exponentially with the size of the system $L$, i.e., $\mathcal{O}(d^L)$. The MPS method is to retain only the first $\chi$ singular values and their corresponding singular vectors in the SVD of the tensor, $\chi$ is known as the truncation dimension. As a result, the size of the dimension $s_l$ on the right-hand side in Eq. S5 becomes $\chi$, and the complexity of its representation of the quantum state is greatly reduced to grow linearly, i.e., $O(Ld\chi^2)$.

In fact, the tensor product representation itself does not have any redundant information, and for an arbitrary many-body state, the information it contains grows exponentially with the number of lattice points $L$. Fortunately, real system interactions tend to be localized, and such localized interactions are manifested in the exponential decay of the correlation function, in addition to the entanglement entropy of their ground and low excited states satisfying the area law, which for a one-dimensional system manifests itself as essentially the same entanglement entropy for the dichotomous system everywhere in the middle. Therefore, in our work (one-dimensional near-neighbor interaction spin chains), quantum states can be characterized in the form of MPS with smaller truncation dimension $\chi$ without loss of generality. Here, we set the truncation dimension $\chi$ to 16.

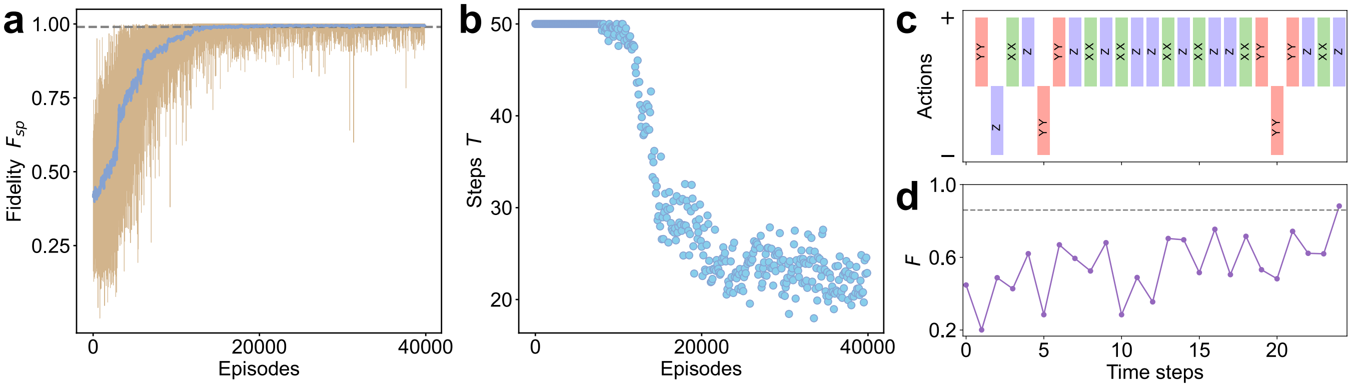


FIG. S3. Training results for preparing the critical ground state of the XY model. (a) Single-particle fidelity $F_{sp}$ of the target ground state during training versus the number of episodes that have been trained. The blue line is the fidelity profile after averaging 100 training episodes, the yellow line is the result without averaging, and the single-particle fidelity threshold $F^*_{\text{sp}} = 0.994$ is marked by the grey dashed line. (b) The number of control actions used to prepare the target state during training versus the number of training rounds, where the maximum number of actions set to 50. (c) Sequence of gates required for the complete control scheme, where the positive (negative) sign on the y-axis indicates the duration of the corresponding actions as positive (negative) time. (d) Total fidelity $F$ of the target state as a function of the number of times (number of gates), and the fidelity threshold $F^* = 0.84$ is marked by the black dashed line.

## IV. EFFECT OF PROBE FIDELITY ON ACTUAL SENSING ACCURACY

In this section, we analyse the effect of the fidelity of the probe on the theoretical sensing accuracy. Ideally the probe is a ground state $|\varphi(\lambda)\rangle$ of the Hamiltonian $H(\lambda)$, but the states prepared by the scheme given by our RL are

$$|\varphi'(\lambda)\rangle = a\,|\varphi(\lambda)\rangle + b\,|\varphi_\perp(\lambda)\rangle\,, \tag{S6}$$

where $\left|a^2\right| = F^*$ is the target fidelity and $|\varphi_\perp(\lambda)\rangle$ lies in excited states space orthogonal to the ground state $|\varphi(\lambda)\rangle$. During the encoding of the unknown parameters, the quantum state evolves adiabatically, i.e., $|\varphi'(\lambda)\rangle \to |\varphi'(\lambda+\delta\lambda)\rangle$. We now recall the Bruce distance formula to calculate the QFI

$$F_Q(\lambda) = \frac{8\left(1 - \left|\langle\varphi(\lambda) \mid \varphi(\lambda+\delta\lambda)\rangle\right|\right)}{\delta\lambda^2}. \tag{S7}$$

Thus for the actual probe $|\varphi'(\lambda)\rangle$, the QFI is

$$F_Q{}'(\lambda) = \frac{8\left(1 - \left|\langle\varphi'(\lambda) \mid \varphi'(\lambda+\delta\lambda)\rangle\right|\right)}{\delta\lambda^2}. \tag{S8}$$

Considering that the excited state space of the many-body system is much less sensitive to parameters near the critical point than the ground state, we have

$$|\varphi_\perp(\lambda)\rangle \approx |\varphi_\perp(\lambda+\delta\lambda)\rangle\,. \tag{S9}$$

Then bringing Eqs. (S6) and (S9) into Eq. (S8), we can obtain the simplified $F'_Q(\lambda)$ as

$$\begin{aligned} F'_Q(\lambda) &\approx 8\left(1 - \left| |a|^2 \langle\varphi(\lambda) \mid \varphi(\lambda+\delta\lambda)\rangle + |b|^2 \right|\right)/\delta\lambda^2 \\ &\approx F^* \cdot F_Q(\lambda) \end{aligned}\,. \tag{S10}$$

Again the average uncertainty versus fidelity can be obtained as

$$\mathcal{K}'_Q = \mathcal{K}_Q / F^*. \tag{S11}$$

Thus, in our work, the effect of the probe fidelity on the sensing accuracy is only linearly reduced.

## V. PREPARATION OF XY MODEL GROUND STATES BY REINFORCEMENT LEARNING

In this section, we demonstrate how to prepare XY model probe with QRL algorithm, and use the ground state with the highest global sensing accuracy ($g_x = 1, \gamma = 0.3$) as an example. Here, the training parameters and action space are kept the same as in the previous Ising model.

In Fig. S3(a) and (b), we show the curve of fidelity of the critical ground state of the QRL preparation XY spin chain ($L = 30$) as it improves with the number of training episodes, as well as the number of actions $T$ used for the preparation versus the number of training episodes. It can be seen that within the maximum number of episodes, the agent gradually prepares the critical ground state with the target fidelity $F^* = 0.84$ and eventually learns the optimal policy during the training process.

In Fig. S3(c) and (d), we show the gate sequences corresponding to the converged QRL scheme and the relationship between the fidelity with the number of gates ($T$) during the preparation of the target ground state of the XY spin chain with $L = 30$. It can be seen that the scheme eventually drives the system to reach the target critical ground state above the threshold $F^*$.

## VI. REALIZATION OF GATE CONTROL IN PHYSICAL SYSTEMS

Realization of complex many-body quantum systems is the way to realize large-scale quantum computation in the future. Current mainstream quantum platforms such as superconducting qubits, neutral atoms, trapped ions, and photons have made good progress [6]. superconducting qubits, neutral atoms, and trapped ions, which are Fermi systems with natural advantages and practical significance in modeling spin systems, have been proved to be promising platforms for solving the strongly correlated many-body phenomena [7–9], and have become the common devices for executing quantum programming and computation in the NISQ era [10, 11]. Among them, superconducting qubits are man-made atoms with advantages such as high integration [12] and long coherence time [13], neutral atoms have the advantages of long coherence time [14], easy manipulation [15], and micrometer-scale interactions [16], and trapped ions have the advantages of high-fidelity preparation and readout [17], long trapping time [18], and high programmability [19]. In this section, we introduce how to implement the gate control in Eq. (S3) employed by QRL on the superconducting qubits, neutral atoms, and trapped ions platform.

First we briefly introduce the Superconducting qubits. Superconducting quantum systems are naturally suited for the implementation of digital quantum simulations, allowing for the precise realization of single and two-site gates.

In superconducting system, where each transmon is a qubit, the arbitrary single-site rotating gates $\{X, Y, Z\}$ can be realized by using controlled voltage pulses to individually adjust the magnetic flux of each qubit. The neighboring transmons can be coupled to the resonator to generate exchange coupling $\sigma_i^x\sigma_{i+1}^x + \sigma_i^y\sigma_{i+1}^y$, and the two-site gates $\{XX, YY, ZZ\}$ can be generated by using a single-site rotating gate before and after the exchange coupling [12].

Then, we introduce the neutral atoms, i.e., the Rydberg atoms platform, which has successfully demonstrated critical sensing with an precision enhancement of the order of $10^3$ [20]. We begin by recalling the most common simulation of the Ising model with an array of Rydberg atoms [21], which Hamiltonian is

$$H_{Ising}^R = \Omega(t)\sum\nolimits_i \sigma_i^x - \Delta(t)\sum\nolimits_i \sigma_i^z + \sum\nolimits_{i<j} V_{ij}\sigma_i^z\sigma_j^z, \tag{S12}$$

where $\Omega(t)$ is the intensity of the Rydberg global laser, $\Delta(t)$ is the detuning of the laser frequency from the Rydberg transition frequency, and $V_{ij}$ is the interaction strength, induced by the van-der-Waals force between the two atoms with space distance $d_{ij}$. In this case, different atoms are excited in the same Rydberg level and the coupling effect between them is second order i.e., $V_{ij} \sim 1/d_{ij}^6$ [22]. By adjusting the intensity and frequency of the laser through techniques such as pulse engineering, arbitrary rotation of atoms in local space can be realized. In addition, considering the power-law decay of the van-der-Waals force, non-nearest neighbor interactions can be neglected and the interaction Hamiltonian can be written as $\sum_i V\sigma_i^z\sigma_{i+1}^z$. Noting the high stability of the Rydberg atoms, the position can be moved by optical tweezers, and thus $V$ is tunable. Therefore, for single-site gates $\{X, Y, Z\}$, they can be achieved by adjusting the position of atoms to turn off the coupling and then adjusting the pulse. For two-site gates, by turning off the laser, only $ZZ$ can be realized in this Hamiltonian model.

Based on the Ising model, it is not yet possible to realize two-site gates $XX$ and $YY$, while the XY model can be realized. The Hamiltonian of the XY model implemented by Rydberg atomic arrays [22] is

$$H_{XY}^R = \sum\nolimits_{i<j} \tilde{V}_{ij}(\sigma_i^x\sigma_j^x + \sigma_i^y\sigma_j^y). \tag{S13}$$

In this case, two atoms are excited in different Rydberg levels and the coupling effect between them is first order i.e., $\tilde{V}_{ij} \sim 1/d_{ij}^3$ [22]. In this model, it is not yet possible to obtain independent two-site gates $\{XX, YY, ZZ\}$ directly, but they can be realized already by Floquet engineering [23]. By applying a periodic laser field, the Hamiltonian is updated as

$$H_{XY}^R(t) = \sum\nolimits_{i<j} \tilde{V}_{ij}(\sigma_i^x\sigma_j^x + \sigma_i^y\sigma_j^y) + H_{drive}(t), \tag{S14}$$

where $H_{drive}(t) = \Omega(t)\sum_i \cos\phi(t)\sigma_i^x + \sin\phi(t)\sigma_i^y$ and $\phi(t)$ is the phase. The single period of $H_{drive}(t)$ is a sequence of four local $\pi/2$ pulses $(X, -Y, Y, -X)$ with delay times $(\tau_1, \tau_2, 2\tau_3, \tau_2)$ respectively. According to the average Hamiltonian theory [24], the time-dependent periodic Hamiltonian $H_{XY}^R(t)$ can be rewritten as the time-independent Hamiltonian:

$$H_{XYZ}^R = \frac{2}{3}\sum\nolimits_{i<j} \tilde{V}_{ij}(c_1\sigma_i^x\sigma_j^x + c_2\sigma_i^y\sigma_j^y + c_3\sigma_i^z\sigma_j^z), \tag{S15}$$

i.e., the XYZ model, where $c_i = \frac{3-\tau_i}{2}$. In this model, if only the nearest-neighbor effect is considered, two-site gates $\{XX, YY, ZZ\}$ can be realized by adjusting the pulse delay times $\tau_i$.

In addition, the recently reported work directly constructs the XYZ model by two-color Rydberg dressing [25, 26], which allows one to engineer the spin-spin couplings in each spin direction by the choice of the laser parameters. The Hamiltonian of this model is

$$H_{XYZ}^R = \sum\nolimits_{i<j} (J_{ij}^z\sigma_i^x\sigma_j^x + J_{ij}^{++}\sigma_i^+\sigma_j^+ + J_{ij}^{+-}\sigma_i^+\sigma_j^-) + \text{H.c.}, \tag{S16}$$

where $J_{ij}^k$ is related to the atomic distance, energy level gap and laser frequency. Therefore, $ZZ$ gate can be realized when $J_{ij}^{++} = J_{ij}^{+-} = 0$, and $XX$ or $YY$ can be realized when $J_{ij}^z = 0, J_{ij}^{++} = J_{ij}^{+-}$ or $J_{ij}^{++} = -J_{ij}^{+-}$.

In addition to superconducting qubits and neutral atoms, trapped ions are currently considered promising platforms for realizing large-scale quantum computation. We now introduce how to realize the gate control we employ in the trapped ions platform by simple laser pulses. The Hamiltonian of a trapped ions chain exposed to multiple beams of uniform laser light with different orientations $(\alpha = x, y, z)$ is given by [27]

$$\begin{aligned} H &= H_\nu + H_f + H_m, \\ H_\nu &= \sum_{\alpha,n} \omega_n^\alpha a_n^{\alpha,+} a_n^\alpha, \\ H_f &= \sum_{\alpha,i,n} F^\alpha \mathcal{M}_{i,n}^\alpha (a_n^\alpha + a_n^{\alpha,+})(1+\sigma_i^\alpha)/\sqrt{2m\omega_n^\alpha}, \\ H_m &= \sum_{\alpha,i} b^\alpha \sigma_i^\alpha, \end{aligned} \tag{S17}$$

where $H_\nu$ is the phonon $n$-mode vibrational Hamiltonian due to Coulomb repulsion, $H_f$ is due to the spin-dependent optical dipole force $F^\alpha$, and $H_m$ is the effective magnetic field term simulated by the laser-induced internal transition of the ions.

The XYZ model can be realized after canonical transformation [28] of the above Hamiltonian, i.e.,

$$\begin{aligned} H_{XYZ}^{Ion} &= e^{-S} H^{Ion} e^{S} \\ &= H_\nu + \tfrac{1}{2}\sum_{a,i,j} J_{ij}^{\alpha}\sigma_i^\alpha\sigma_j^\alpha + \sum_{\alpha,i} B^\alpha\sigma_i^\alpha + H_E \ , \end{aligned} \tag{S18}$$

where

$$S = \sum_{\alpha,i,n} \eta_{in}^{\alpha}(a_n^{\alpha,+} - a_n^{\alpha})(1+\sigma_i^\alpha), \quad \eta_{in}^{\alpha} = \frac{F^\alpha \mathcal{M}_{i,n}^{\alpha}}{\omega_n^\alpha\sqrt{2m\omega_n^\alpha}}. \tag{S19}$$

In Eq. (S18) The coupling term $H_E$ is a perturbation and can be neglected in the phonon low temperature case. Thus the phonon degrees of freedom are decoupled from the spin degrees of freedom, and we can obtain the standard XYZ Hamiltonian

$$H_{XYZ}^{Ion} = \frac{1}{2}\sum_{\alpha,i,j} J_{ij}^{\alpha}\sigma_i^\alpha\sigma_j^\alpha + \sum_{\alpha,i} B^\alpha\sigma_i^\alpha, \tag{S20}$$

where the coupling coefficient $J_{ij}^\alpha \sim 1/d_{ij}^3$ and the effective magnetic field strength $B^\alpha = b^\alpha - (F^\alpha)^2/m(\omega^\alpha)^2$. Notice that their coupling coefficient $J_{ij}^\alpha$ is power-law decaying, so the non-nearest neighbor coupling can be neglected. The whole Hamiltonian depends on the laser number, direction $\alpha$, frequency $\omega^\alpha$, and distance $d_{i,i+1}$ of ions. Therefore experimentally selecting a laser with a fixed direction and adjusting its frequency and alignment distance of ions, an arbitrary gate in the set $\{X, Y, Z, XX, YY, ZZ\}$ can be realized.

## VII. TRANSLATION INVARIANCE OF THE MANY-BODY SYSTEM

Here we take the Ising model as an example to analyze the translation invariance of the many-body ground state. First we recall the Hamiltonian of the Ising model as shown in Eq. (S23). Since each lattice point corresponds to the same operator, i.e., translational invariance, it can be conjectured that the reduced density matrix and entanglement spectrum of its ground states are also the same at each lattice point. To verify this, we give in Fig. S4 the properties of the critical ground states of the Ising model at different sizes. In Fig. S4, the Pauli expectation values $\langle\sigma_i^k\rangle$ reflect the reduced density matrices $\rho_i$ of the individual spins on lattice point $i$, i.e.,

$$\rho_i = \left( I + \sum_{k=x,y,z} \langle\sigma_i^k\rangle \cdot \sigma_i^k \right) \Big/ 2. \tag{S21}$$

The $M_i^{two}$ is the mutual information of the spins of neighboring lattice points $i$ and $i+1$, which measures their entanglement. The mutual information can be expressed as

$$M_i^{two} = S(\rho_i) + S(\rho_{i+1}) - S(\rho_{i,i+1}), \tag{S22}$$

where $S(\rho_i)$ and $S(\rho_{i,i+1})$ are the von Neumann entropy of the density matrices of a single spin and two neighboring spins, respectively. It is easy to see that when $L$ is fixed, the states and entanglements on different lattice points are almost the same. The open boundary conditions of the spin model lead to different spin properties at the edges, which is called the boundary effect. When $L$ increases, excluding the boundary effect, the state and entanglement of individual lattice points do not change, which we confirm in Fig. S5(a). We can therefore infer that the local properties of the translation invariant many-body ground state are independent of $L$, i.e., size invariance. A more intuitive understanding of size invariance is that due to the local entanglement properties of the system, the added spins do not change the spins that are farther away, and when the size is sufficiently large, excluding the spins at the edges, all the other spins tend to stabilize and do not change with size $L$.

We now analyze the utility of the control actions we employ as shown in Eq. (S3). The single-site gate only changes the spin direction at each lattice point, and it is easy to see that its effect is size invariant, since the angle of rotation is independent of size. The two-site gates generate entanglement or disentanglement, again with size invariance, which can be reflected in Fig. S5(b). Thus if a gate sequence can prepare a critical ground state with size invariance, it can necessarily be expanded to any size, since the gate sequence also has size invariance.

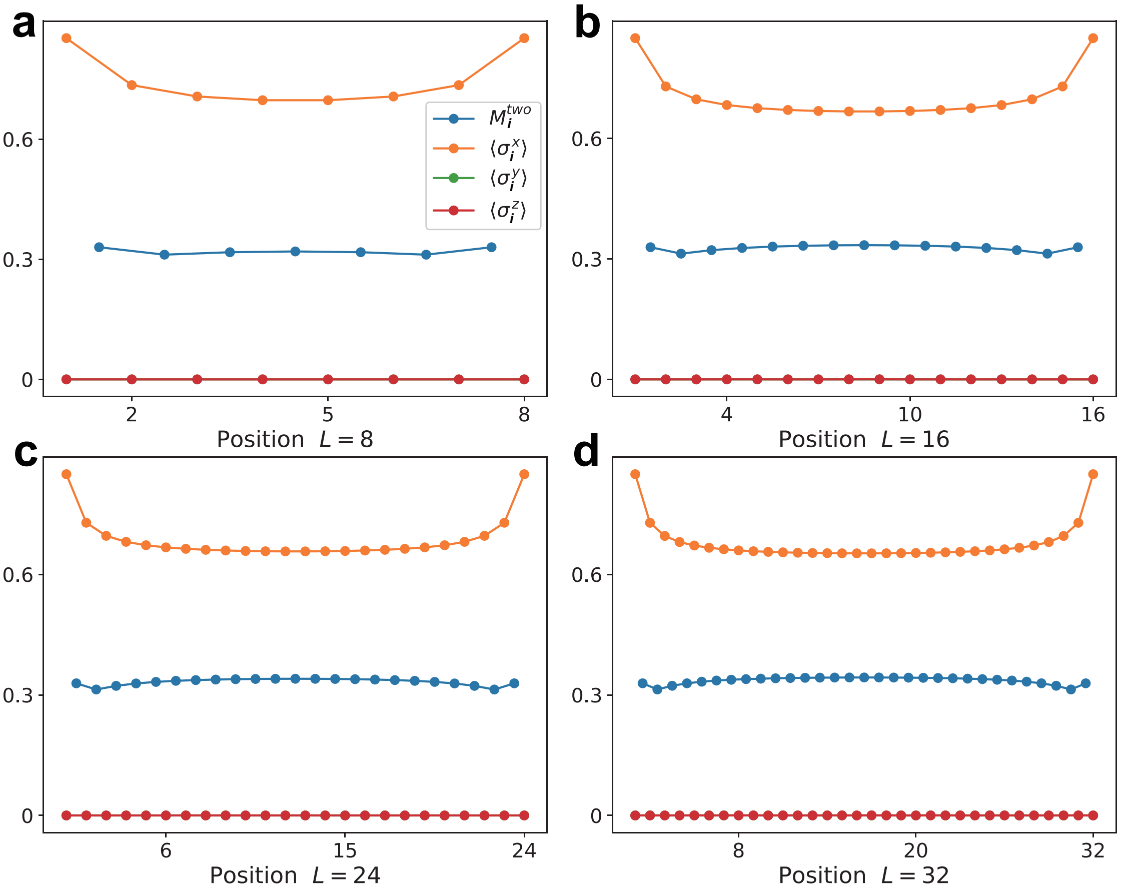


FIG. S4. Properties of individual spins of the Ising model at different sizes $L$ with respect to the position $i$ of the lattice points.

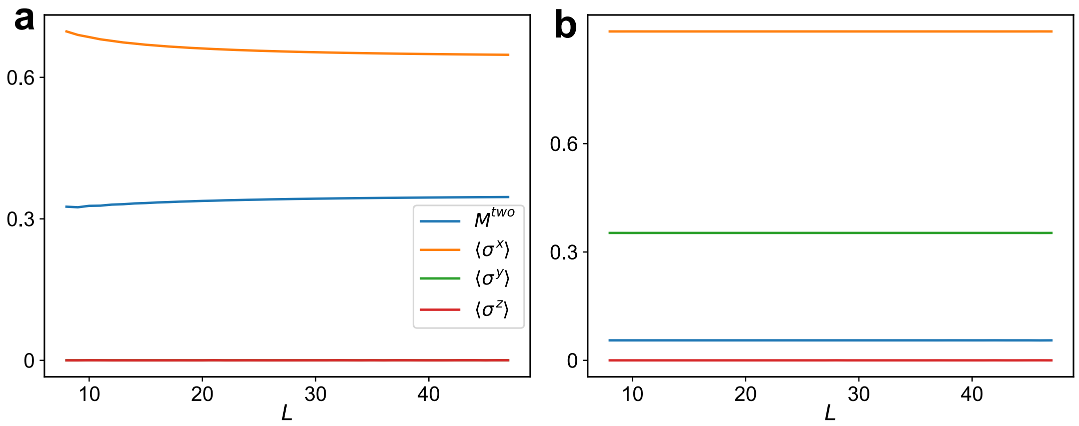


FIG. S5. (a) Properties of the central spin of the Ising critical ground state versus the system size. (b) Properties of the central spin after a set of two-site gates acting on a product state versus the size of the system.

In Fig. S6, we show the generalizability of the gate sequences obtained by training at different sizes $L$. Here, the different curves correspond to different gate sequences, but each curve is the result obtained by uniformly applying the same gate sequence to spin systems with different size $L$. The different training models are better able to prepare critical ground states of larger sizes, however the models obtained by training on larger sizes are better. The translation invariance ensures that the gate sequences obtained by training at a specific size can be generalized to any size, but the performance of the gate sequences obtained by training at different sizes are all different. This is mainly due

to the asymptotic property of translation invariance, which holds only in the thermodynamic limit ($L \to \infty$) and is only approximately valid for small-scale systems. Therefore, if computational resources are available, we suggest that training on a large scale makes it possible to obtain gate sequences in the thermodynamic limit that generalize well to arbitrary sizes $L$.

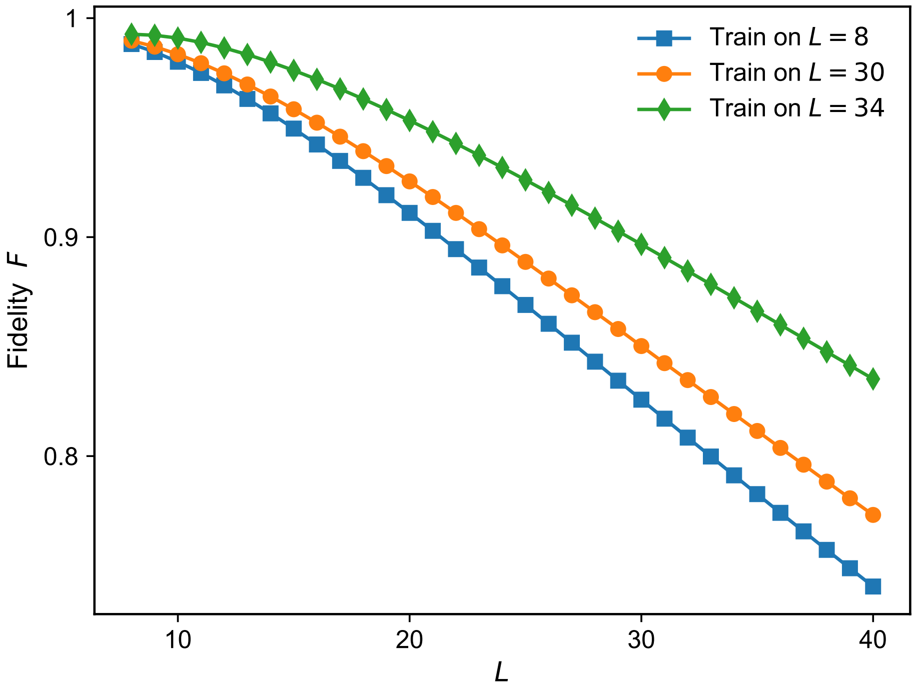


FIG. S6. Generalizability of gate sequence for different trained models.

## VIII. ADDITIONAL INTRODUCTION TO THE ISING MODEL

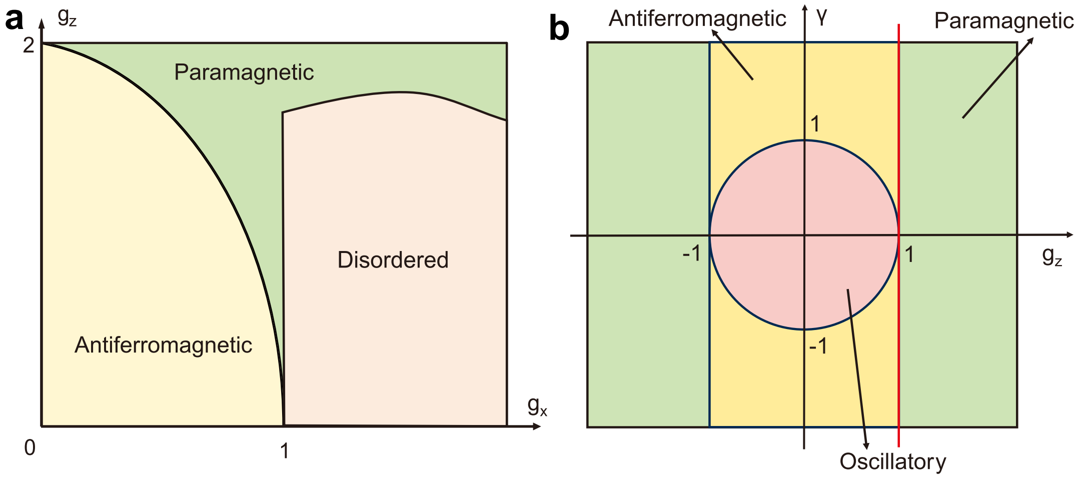


FIG. S7. Ground-state phase diagram of the Ising (a) and XY (b) model in parameter plane.

The Hamiltonian of the Ising spin chain system interacting with the control magnetic field $\boldsymbol{B}$ and the measured

magnetic field $\boldsymbol{h}$ is

$$H_{Ising} = J\sum_{i=1}^{L-1}\sigma_i^z\sigma_{i+1}^z + g_x\sum_{i=1}^{L}\sigma_i^x + g_z\sum_{i=1}^{L}\sigma_i^z, \tag{S23}$$

where $\boldsymbol{g} = \boldsymbol{B}+\boldsymbol{h}$ is the total magnetic field strength. In Fig. S7(a), we plot the phase diagram [29] of this Hamiltonian on the parameter space $(g_x, g_z)$, and we use the ground state $(g_x = 1, g_z = 0)$ at the boundary between paramagnetic and antiferromagnetic as the sensing probe.

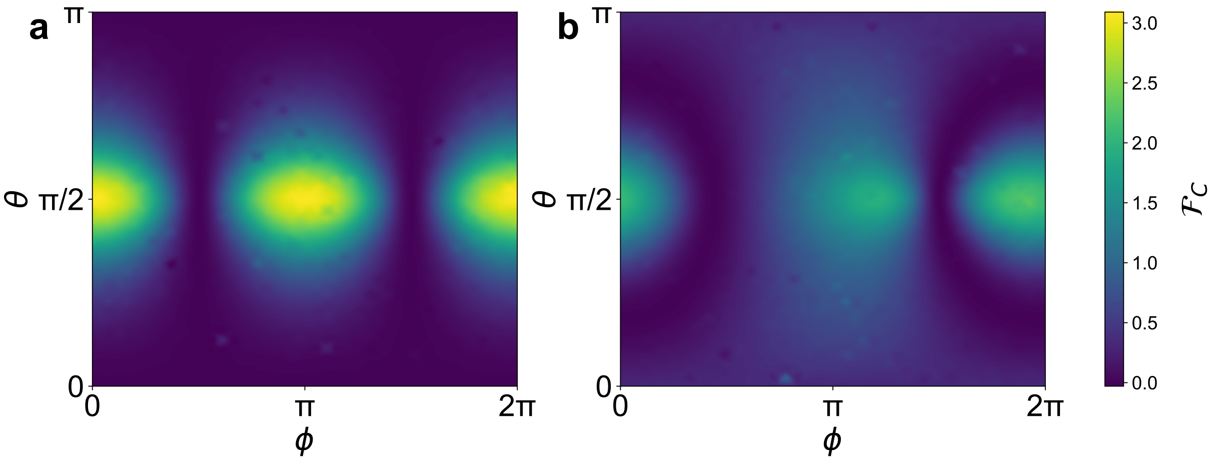


FIG. S8. CFI $F_C$ of the critical ground state ($L = 8$) of the Ising model on different measurement bases. (a) CFI of one-site measurements with different Bloch sphere parameters in Eq. (S24). (b) CFI of two-site measurements with different Bloch sphere parameters.

we use the critical ground state ($g_x$=1, $g_z$=0) of the model as a sensing probe to probe the $x$-component of the magnetic field $h_x$ (single-parameter estimation) and it turns out that its characterization by QFI is accurate up to the Heisenberg limit. Now, we analyze its measurement-based CFI. Considering the feasibility of practical measurements, the choice is between single ($\mathcal{O}_{single} = \sum_{i=1}^{L}\boldsymbol{\sigma}_i$) and two-site measurements ($\mathcal{O}_{two} = \sum_{i=1}^{L-1}\boldsymbol{\sigma}_i\boldsymbol{\sigma}'_{i+1}$) is sensible. Here $\boldsymbol{\sigma}_i$ denotes a direction-specific Pauli operator:

$$\boldsymbol{\sigma}_i = \sigma_i^z\cos\theta + \sigma_i^x\sin\theta\cos\phi + \sigma_i^y\sin\theta\sin\phi. \tag{S24}$$

Notice that when $\boldsymbol{\sigma}_i = \boldsymbol{\sigma}'_{i+1}$ in the two-site measurement, its CFI is the same as that under one-site measurement $\sum_{i=0}^{L}\boldsymbol{\sigma}_i$. This is because at this point $\left[\sum_{i=0}^{L}\boldsymbol{\sigma}_i, \sum_{i=1}^{L-1}\boldsymbol{\sigma}_i\boldsymbol{\sigma}_{i+1}\right] = 0$, and they share the same set of eigenstates. Therefore, we choose different $\boldsymbol{\sigma}_i$ vs. $\boldsymbol{\sigma}'_{i+1}$ for the two-site measurement, and here we fix $\boldsymbol{\sigma}'_{i+1}$=$\sigma^y_{i+1}$.

In Fig. S8(a) and (b), we plot the thermodynamic diagrams of CFI under different single-site measurement bases and two-site measurement bases, respectively. It is clear from the plots that the optimal measurement basis is the global magnetization $\sum_{i=0}^{L}\sigma_i^x$. This result is of great significance for our study because one-site measurements are easier to implement than two-site measurements, which makes them more convenient and efficient in practical applications. In Fig. S9, we plot the time-factorized CFI and CFI-based average uncertainty of QRLCS versus spin length $L$ under different measurement bases, respectively. It can be shown that the sensing accuracy of our protocol on these measurement bases reaches the sub-Heisenberg limit for both the local and global cases. In addition the optimal measurement basis is the single-one measurement $\sum_{i=0}^{L}\sigma_i^x$, while the other measurements have only a slight disadvantage.

## IX. ADDITIONAL INTRODUCTION TO THE XY MODEL

The phase diagram [30] of the XY model of the ground state in the parameter space $(g_x, \gamma)$ is given by Fig. S7(b). In the main text we use the ground state on the line $g_z = 1$ as the sensing probe. However, different ground states on this straight line have different critical exponents, which can lead to different sensitivities. For this reason, we need to analyze the sensitivity of the critical ground state for different $\gamma$. In Fig. S10(a),(b) we plot QFI and average

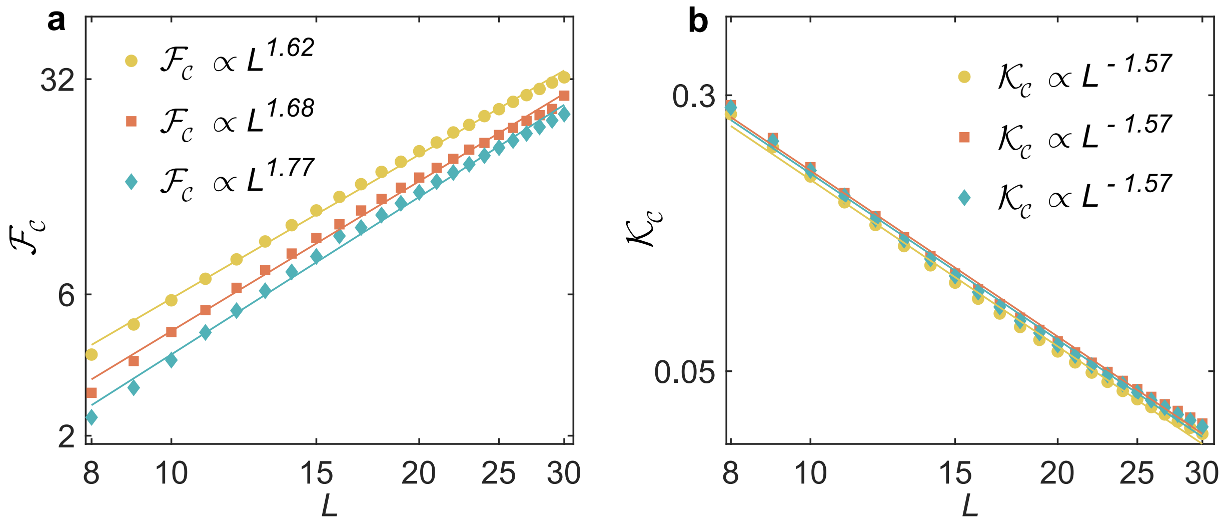


FIG. S9. Sensing performance characterized by CFI of QRLCS for the Ising model. (a) Time-factorized CFI $\mathcal{F}_\mathcal{C}$ as a function of spin chain length $L$ under different measurement bases in the local sensing case. (b) Average uncertainty $\mathcal{K}_\mathcal{C}$ as a function of spin chain length $L$ under different measurement bases in the global sensing case, where $\Delta h_x = 0.1$.

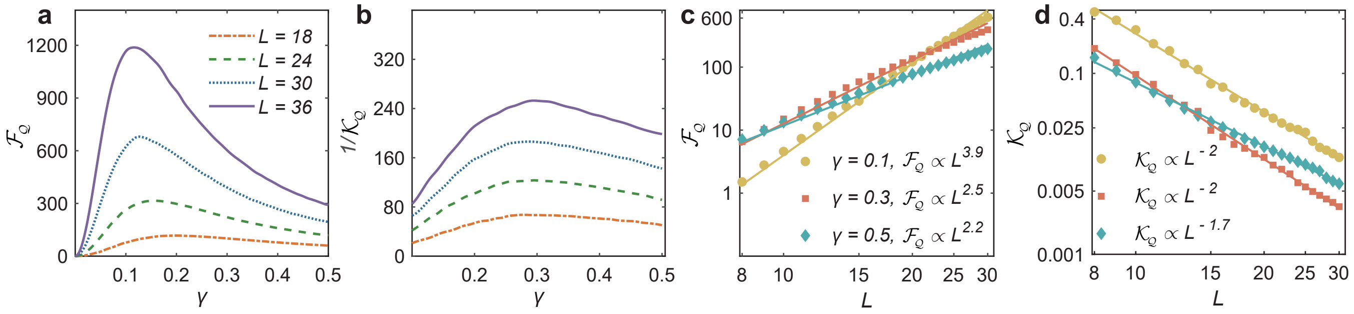


FIG. S10. Sensing performance of the XY model. (a) Time-factorized QFI $\mathcal{F}_\mathcal{Q}$ as a function of the anisotropic parameter $\gamma$ chain for different length $L$ of spin in critical line $g_z = 1$. (b) The inverse of the average uncertainty $1/\mathcal{K}_\mathcal{Q}$ as a function of the anisotropic parameter $\gamma$ chain for different length $L$ of spin in critical line $g_z = 1$. (c) Time-factorized QFI $\mathcal{F}_\mathcal{Q}$ as a function of length $L$ of spin chain for different values of the anisotropic parameter $\gamma$ and same transverse field $g_z = 1$ in the local sensing case. In this case the critical probe ($\gamma = 0.1$, yellow dots) reaches the super-Heisenberg limit, while the others are roughly in the Heisenberg limit. (d) Average uncertainty $\mathcal{K}_\mathcal{Q}$ as a function of length $L$ of spin chain for different values of the anisotropic parameter $\gamma$ and same transverse field $g_z = 1$ in the global sensing case, where $\Delta h_z = 0.1$. In this case the critical probes ($\gamma = 0.1$, yellow dots; $\gamma = 0.3$, red squares) all reach the Heisenberg limit.

uncertainty versus $\gamma$, respectively, where Fig. S10(a) corresponds to the local sensing case and Fig. S10(b) corresponds to global sensing with a dynamic range width of 0.1. It can be seen that as the system scale increases, the values of $\gamma$ corresponding to the highest sensing accuracy converge towards 0.1 and 0.3 out, respectively. Therefore, it can be expected that the base state probes corresponding to these two points should be the optimal probes for local and global sensing, respectively.

In Fig. S10(c), we plot the time-factorized QFI of the XY model probe as a function of the spin chain length $L$ for different parameters $\gamma$. It can be seen that for local sensing, the same is the critical ground state which is located on the straight line $g_z = 1$ in the parameter space, but the sensing accuracy corresponding to the different parameters $\gamma$ is different, in which the ground state at $\gamma = 0.1$ reaches the super-Heisenberg limit, and the Heisenberg limit in other cases. In Fig. S10(d), we plot the average uncertainty of the XY model probe as a function of the spin chain length $L$ for different parameters $\gamma$. It can be seen that for global sensing with a dynamic range of 0.1, the sensing accuracy of the critical ground state at $\gamma = 0.1$ degrades to the Heisenberg limit, whereas the absolute accuracy of the critical ground state at $\gamma = 0.3$ is instead higher than the former, despite the fact that it maintains the Heisenberg limit.

Similarly, we need to analyze the CFI of the XY model under different measurement bases. Considering the same type of measurement bases as the Ising model, we give its CFI versus the measurement base parameters in Fig. S11. It can be seen that the optimal measurement within the set of single- and two-site measurements is the single-site

collective $z$-spin measurement (corresponding to the straight line $\theta = 0$ or $\pi$ in Fig. S11(a)). Next, we evaluate the actual accuracy given by the measurement data for the critical probe of the model under different measurement bases. As shown in Fig. S12, for both probes $\gamma = 0.1$ and $\gamma = 0.3$, it remains the case that the local case $\gamma = 0.1$ outperforms $\gamma = 0.3$, while the global case $\gamma = 0.3$ outperforms $\gamma = 0.1$. For the local case, the performance under different measurement bases is indeed optimal for the collective $z$-spin measurements, which is in agreement with the conclusions inferred from Fig. S11.

For the MXY model, considering that its critical ground state is the same as that of XY, the sensitivity of its critical ground state under different $\gamma$ and the comparison of the accuracy under different measurements are not analyzed here, while the results of these comparisons are in fact consistent with that of the XY model. However, it is additionally important to add that although the critical probes of the two models are the same, they undergo different parameter encoding processes. the special coupling of the MXY model provides a more complex critical region, and thus the trend of the quantum state within a specific parameter interval is more pronounced, leading to its higher parameter estimation accuracy.

Finally, it should be added that for the noise cases considered in the main text. These noises can affect the fidelity of the QRL-prepared critical probes and ultimately the actual sensing accuracy. In Fig. S13, we give the probe fidelity versus spin length $L$ for different noise scenarios. It can be seen that the effect of noise on the fidelity of the probe is roughly $2 \sim 10\%$, which increases with $L$.

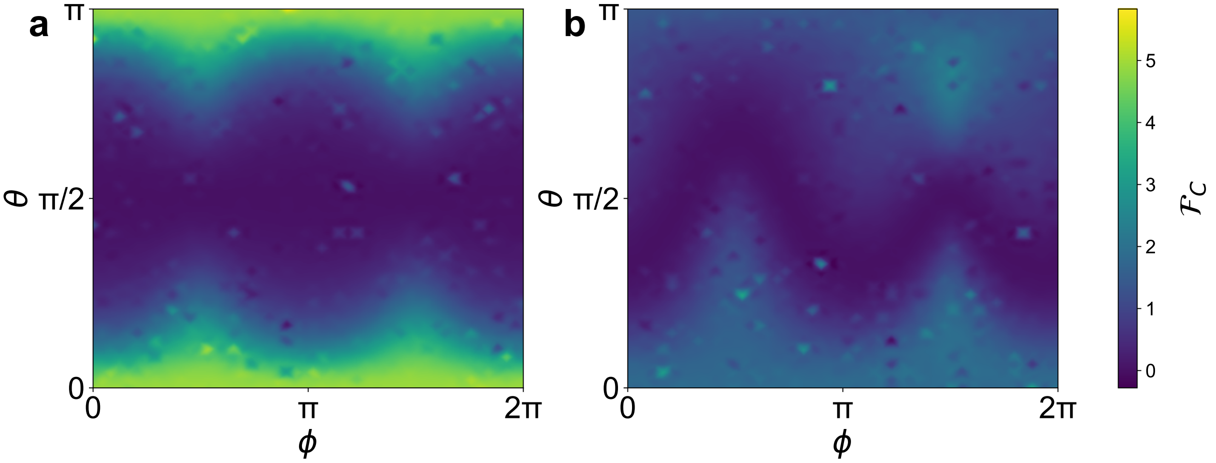


FIG. S11. CFI $F_C$ of the critical ground state ($\gamma = 0.3, L = 8$) of the XY model on different measurement bases. (a) CFI of one-site measurements with different Bloch sphere parameters in Eq. (S24). (b) CFI of two-site measurements with different Bloch sphere parameters.

[1] V. Mnih, K. Kavukcuoglu, D. Silver, A. A. Rusu, J. Veness, M. G. Bellemare, A. Graves, M. Riedmiller, A. K. Fidjeland, G. Ostrovski, *et al.*, Human-level control through deep reinforcement learning, Nature **518**, 529 (2015).
[2] H. Van Hasselt, A. Guez, and D. Silver, Deep reinforcement learning with double q-learning, in *Proceedings of the AAAI conference on artificial intelligence*, Vol. 30 (2016).
[3] N. Schuch, M. M. Wolf, F. Verstraete, and J. I. Cirac, Entropy scaling and simulability by matrix product states, Physical Review Letters **100**, 030504 (2008).
[4] S. R. White, Density matrix formulation for quantum renormalization groups, Physical Review Letters **69**, 2863 (1992).
[5] S. Östlund and S. Rommer, Thermodynamic limit of density matrix renormalization, Physical Review Letters **75**, 3537 (1995).
[6] I. M. Georgescu, S. Ashhab, and F. Nori, Quantum simulation, Reviews of Modern Physics **86**, 153 (2014).
[7] C. Gross and I. Bloch, Quantum simulations with ultracold atoms in optical lattices, Science **357**, 995 (2017).
[8] R. Blatt and C. F. Roos, Quantum simulations with trapped ions, Nature Physics **8**, 277 (2012).
[9] B. P. Lanyon, C. Hempel, D. Nigg, M. Müller, R. Gerritsma, F. Zähringer, P. Schindler, J. T. Barreiro, M. Rambach, G. Kirchmair, *et al.*, Universal digital quantum simulation with trapped ions, Science **334**, 57 (2011).
[10] M. Morgado and S. Whitlock, Quantum simulation and computing with Rydberg-interacting qubits, AVS Quantum Science **3** (2021).

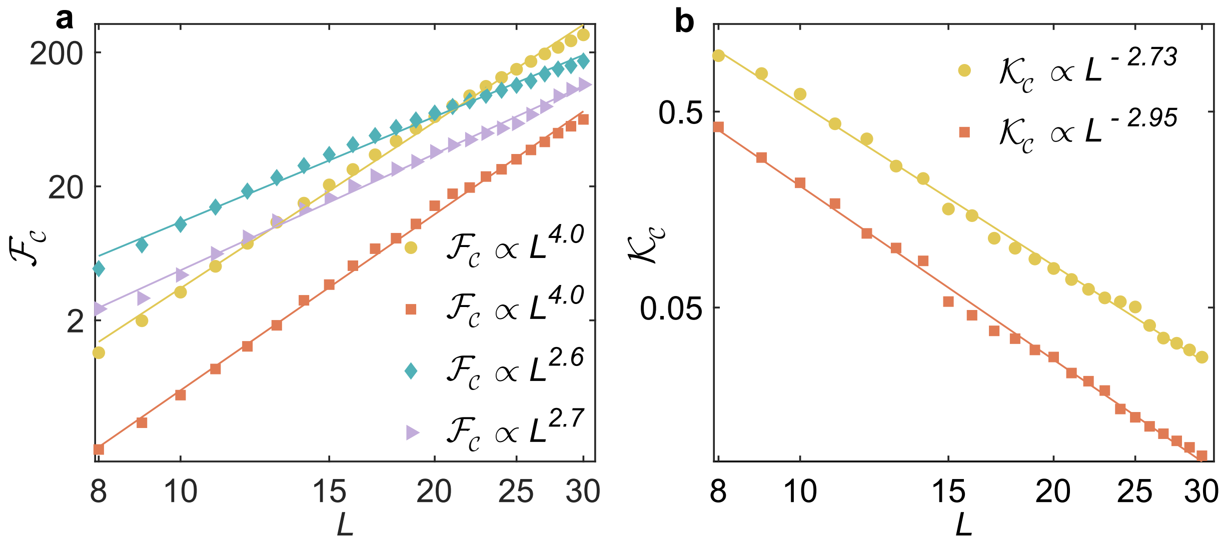


FIG. S12. Sensing performance characterized by CFI of QRLCS for the XY model. (a) Time-factorized QFI $\mathcal{F}_\mathcal{C}$ as a function of spin chain length $L$ under different measurement bases in the local sensing case. (b) Average uncertainty $\mathcal{K}_\mathcal{C}$ as a function of spin chain length $L$ under optimal measurement basis in the global sensing case, where $\Delta h_x = 0.1$.


[11] Y. Wu, W.-S. Bao, S. Cao, F. Chen, M.-C. Chen, X. Chen, T.-H. Chung, H. Deng, Y. Du, D. Fan, *et al.*, Strong quantum computational advantage using a superconducting quantum processor, Physical Review Letters **127**, 180501 (2021).

[12] Y. Salathé, M. Mondal, M. Oppliger, J. Heinsoo, P. Kurpiers, A. Potočnik, A. Mezzacapo, U. Las Heras, L. Lamata, E. Solano, *et al.*, Digital quantum simulation of spin models with circuit quantum electrodynamics, Physical Review X **5**, 021027 (2015).

[13] J. M. Chow, A. D. Córcoles, J. M. Gambetta, C. Rigetti, B. R. Johnson, J. A. Smolin, J. R. Rozen, G. A. Keefe, M. B. Rothwell, M. B. Ketchen, *et al.*, Simple all-microwave entangling gate for fixed-frequency superconducting qubits, Physical Review Letters **107**, 080502 (2011).

[14] M. A. Norcia, A. W. Young, W. J. Eckner, E. Oelker, J. Ye, and A. M. Kaufman, Seconds-scale coherence on an optical clock transition in a tweezer array, Science **366**, 93 (2019).

[15] A. M. Kaufman and K.-K. Ni, Quantum science with optical tweezer arrays of ultracold atoms and molecules, Nature Physics **17**, 1324 (2021).

[16] E. Urban, T. A. Johnson, T. Henage, L. Isenhower, D. Yavuz, T. Walker, and M. Saffman, Observation of Rydberg blockade between two atoms, Nature Physics **5**, 110 (2009).

[17] T. Harty, D. Allcock, C. J. Ballance, L. Guidoni, H. Janacek, N. Linke, D. Stacey, and D. Lucas, High-fidelity preparation, gates, memory, and readout of a trapped-ion quantum bit, Physical Review Letters **113**, 220501 (2014).

[18] D. Kielpinski, C. Monroe, and D. J. Wineland, Architecture for a large-scale ion-trap quantum computer, Nature **417**, 709 (2002).

[19] C. D. Marciniak, T. Feldker, I. Pogorelov, R. Kaubruegger, D. V. Vasilyev, R. van Bijnen, P. Schindler, P. Zoller, R. Blatt, and T. Monz, Optimal metrology with programmable quantum sensors, Nature **603**, 604 (2022).

[20] D.-S. Ding, Z.-K. Liu, B.-S. Shi, G.-C. Guo, K. Mølmer, and C. S. Adams, Enhanced metrology at the critical point of a many-body Rydberg atomic system, Nature Physics **18**, 1447 (2022).

[21] D. Bluvstein, A. Omran, H. Levine, A. Keesling, G. Semeghini, S. Ebadi, T. T. Wang, A. A. Michailidis, N. Maskara, W. W. Ho, *et al.*, Controlling quantum many-body dynamics in driven Rydberg atom arrays, Science **371**, 1355 (2021).

[22] A. Browaeys and T. Lahaye, Many-body physics with individually controlled Rydberg atoms, Nature Physics **16**, 132 (2020).

[23] S. Geier, N. Thaicharoen, C. Hainaut, T. Franz, A. Salzinger, A. Tebben, D. Grimshandl, G. Zürn, and M. Weidemüller, Floquet hamiltonian engineering of an isolated many-body spin system, Science **374**, 1149 (2021).

[24] A. Brinkmann, Introduction to average Hamiltonian theory. I. Basics, Concepts in Magnetic Resonance Part A **45**, e21414 (2016).

[25] A. W. Glaetzle, M. Dalmonte, R. Nath, C. Gross, I. Bloch, and P. Zoller, Designing frustrated quantum magnets with laser-dressed Rydberg atoms, Physical Review Letters **114**, 173002 (2015).

[26] L.-M. Steinert, P. Osterholz, R. Eberhard, L. Festa, N. Lorenz, Z. Chen, A. Trautmann, and C. Gross, Spatially tunable spin interactions in neutral atom arrays, Physical Review Letters **130**, 243001 (2023).

[27] D. Porras and J. I. Cirac, Effective quantum spin systems with trapped ions, Physical Review Letters **92**, 207901 (2004).

[28] F. Mintert and C. Wunderlich, Ion-trap quantum logic using long-wavelength radiation, Physical Review Letters **87**, 257904 (2001).

[29] O. d. A. Bonfim, B. Boechat, and J. Florencio, Ground-state properties of the one-dimensional transverse Ising model in

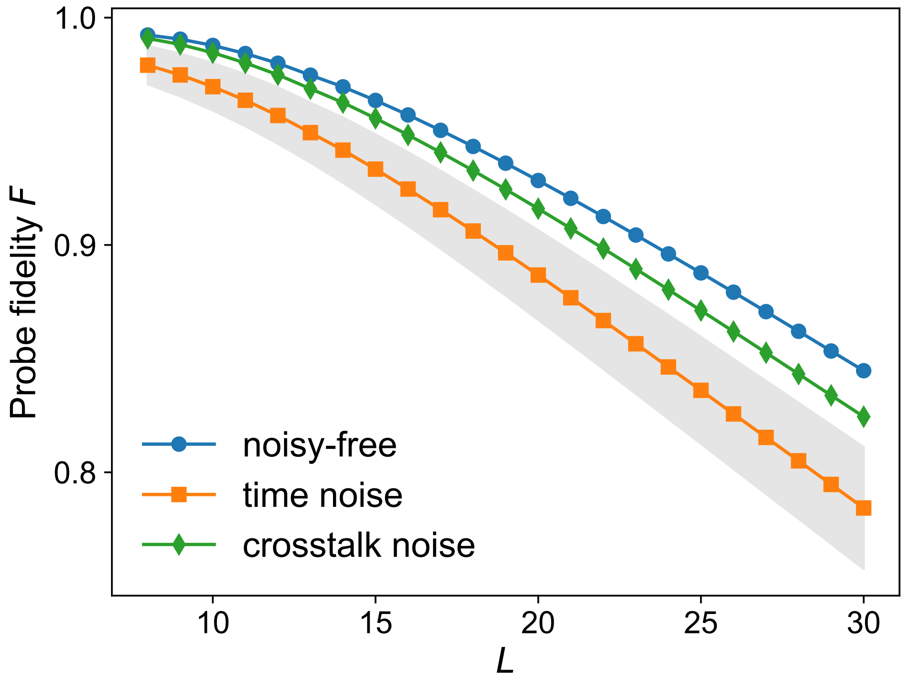


FIG. S13. Fidelity of critical probes versus spin length L in different noise scenarios. The blue line corresponds to the noise free case, the orange line corresponds to the mean of the random time noise, the gray shaded part indicates its standard deviation, and the green line indicates the $ZZ$-coupling crosstalk noise.

a longitudinal magnetic field, Physical Review E **99**, 012122 (2019).

[30] R. Radgohar and A. Montakhab, Global entanglement and quantum phase transitions in the transverse XY heisenberg chain, Physical Review B **97**, 024434 (2018).
